# Supplementary material for: VAPO: Efficient and Reliable Reinforcement Learning for Advanced Reasoning Tasks
Source: arXiv:2504.05118 source file (2025-04-11)
Supplement: Supplementary file 1 [file appendix.tex]

\section{Hello World}
%\subsection{Hello World}
